# Supplementary material for: Finding the Smallest Possible Exact Aggregation of a Markov Chain
Source: arXiv:2507.11157 source file (2025-07-15)
Supplement: Supplementary file 1 [file appendix.tex]

\chapter{Source code}\label{ch:appendix-code}
The used Julia version from~\cite{julia2017} is 1.11.2 and for KrylovKit from~\cite{haegeman2024krylovkit}, version 0.9.4 is used.
Note that these are only the source-files regarding key functionalities.
Things such as input-/output-handling are not shown here.
Lastly, \enquote{Naive arnoldi} refers to the method of aggregation as presented in Definition~\ref{def:arnoldi-aggr}, whereas \enquote{Arnoldi-Schur} refers to the same with the addition of Algorithm~\ref{alg:qralgorithm} at the end to compute the approximated stationary distribution or $\inp{\abs{\pi}, \abs{\mat{\Pi}\mat{A} - \mat{A}\mat{P}} \cdot \mathbf{1}_n}$ as a convergence criterion from Section~\ref{subsec:determining-convergence}.
Lastly, in \enquote{dynamic Arnoldi-Schur} the same is done, but Algorithm~\ref{alg:qralgorithm} is used in a selected number of iterations to determine when to terminate.

\paragraph{algorithms.jl}
\begin{verbatim}
using LinearAlgebra
using KrylovKit


"""
    naive_arnoldi(k::Int, orth::KrylovKit.Orthogonalizer)

Return a function which takes a Markov chain `P` with initial distribution
`p_0` and returns its Arnoldi aggregation of size `k`, using the given
method of orthonormalization `orth`.
"""
function naive_arnoldi(k::Int, orth::KrylovKit.Orthogonalizer)
     return (P::AbstractMatrix, p_0::AbstractVector) ->
                _naive_arnoldi_impl(P, p_0, k, orth)
end

"""
    arnoldi_schur(k::Int, orth::KrylovKit.Orthogonalizer)

Return a function which takes a Markov chain `P` with initial distribution
`p_0` and returns its Arnoldi aggregation of size `k`, using the given
method of orthonormalization `orth`.
Further, the convergence criterion via the Schur decomposition
of `Π` is computed but not applied.
"""
function arnoldi_schur(k::Int, orth::KrylovKit.Orthogonalizer)
     return (P::AbstractMatrix{Float64}, p_0::Vector{Float64}) ->
                            _arnoldi_schur_impl(P, p_0, k, orth)
end

"""
    dynamic_arnoldi_schur(k::Int, orth::KrylovKit.Orthogonalizer)

Return a function which takes a Markov chain `P` with initial distribution
`p_0` and returns its Arnoldi aggregation of size `k`, using the given
method of orthonormalization `orth`.
Further, the convergence criterion via the Schur decomposition
of `Π` is used and actually applied.
"""
function dynamic_arnoldi_schur(k::Int, ε::Float64, step_size::Int64,
                            orth::KrylovKit.Orthogonalizer)
     return (P::AbstractMatrix{Float64}, p_0::Vector{Float64}) ->
                            _dynamic_arnoldi_schur_impl(P, p_0, k, ε,
                                step_size, orth)
end

"""
    _naive_arnoldi_impl(P::AbstractMatrix, p_0::AbstractVector, k::Int,
                orth::KrylovKit.Orthogonalizer)

Compute the aggregated step matrix `Π` of size `k`, disaggregation matrix
`A` and aggregated initial distribution `π_0` by using the Arnoldi
aggregation for a Markov chain `P` and initial distribution `p_0`, using
`orth` as a method of orthonormalization.
"""
function _naive_arnoldi_impl(P::AbstractMatrix, p_0::AbstractVector,
                            k::Int, orth::KrylovKit.Orthogonalizer)
    iterator = ArnoldiIterator(P, p_0, orth)
    factorization = initialize(iterator)
    # Starts with aggregation size 1, so k-1 steps, instead of k
    [expand!(iterator, factorization) for _ in 1:k - 1]
    A = stack(basis(factorization))
    Π = rayleighquotient(factorization)
    π_0 = Float64[norm(p_0, 2); zeros(Float64, k - 1)]
    # Return arbitrary eigenvector as it is not computed with this method
    return Π, A, π_0, π_0
end

"""
    _arnoldi_schur_impl(P::AbstractMatrix, p_0::AbstractVector, k::Int,
                orth::KrylovKit.Orthogonalizer)

Compute the aggregated step matrix `Π` of size `k`, disaggregation matrix
`A` and aggregated initial distribution `π_0` by using the Arnoldi
aggregation for a Markov chain `P` and initial distribution `p_0`, using
`orth` as a method of orthonormalization. Additionally, an aggregated
stationary distribution is computed, using the Krylov-Schur method.
"""
function _arnoldi_schur_impl(P::AbstractMatrix{Float64},
                            p_0::Vector{Float64}, k::Int,
                            orth::KrylovKit.Orthogonalizer)
    # Starts with aggregation size 0, so k steps, instead of k-1
    # The two ones denote no restarts and searching for only one eigenpair
    alg = Arnoldi(orth, k, 1, KrylovDefaults.tol[], false, 1)
    _, U, fact, _, _, _ = KrylovKit._schursolve(P, p_0, 1, :LR, alg)
    A = stack(basis(fact))
    Π = rayleighquotient(fact)
    π_st = @view U[:, 1]
    π_0 = Float64[norm(p_0, 2); zeros(Float64, k - 1)]
    return Π, A, π_st, π_0
end

"""
    _dynamic_arnoldi_schur_impl(P::AbstractMatrix{Float64},
                            p_0::Vector{Float64}, max_size::Int,
                            ε::Float64, orth::KrylovKit.Orthogonalizer)

Compute the aggregated step matrix `Π` of size at most `max_size`,
disaggregation matrix `A` and aggregated initial distribution `π_0` by
using the Arnoldi aggregation for a Markov chain `P` and initial
distribution `p_0`, using `orth` as a method of orthonormalization.
Additionally, an aggregated stationary distribution is computed, using
the Krylov-Schur method. Additionally, the Schur decomposition is
computed every `schur_step_size` steps, to stop if ⟨|π|, |ΠA-AP|⋅1_n⟩
is less than `ε`.

It is simply an adoption of KrylovKit._schursolve().
"""
function _dynamic_arnoldi_schur_impl(P::AbstractMatrix{Float64},
                            p_0::Vector{Float64}, max_size::Int,
                            ε::Float64, schur_step_size::Int64,
                            orth::KrylovKit.Orthogonalizer)
    iter = ArnoldiIterator(P, p_0, orth)
    fact = initialize(iter)
    sizehint!(fact, max_size)
    # preallocate storage
    HH = fill(zero(eltype(fact)), max_size + 1, max_size)
    UU = fill(zero(eltype(fact)), max_size, max_size)
    k = 1   # Current size of Π
    local T, U
    while k < max_size || max_size == 1
        k = length(fact)
        if k % schur_step_size == 0
            H = view(HH, 1:k, 1:k)
            U = view(UU, 1:k, 1:k)
            copyto!(U, I)
            copyto!(H, rayleighquotient(fact))
            # compute dense schur factorization
            T, U, values = KrylovKit.hschur!(H, U)
            by, rev = KrylovKit.eigsort(:LR)
            p = sortperm(values; by=by, rev=rev)
            T, U = KrylovKit.permuteschur!(T, U, p)
            # Compute convergence criterion
            A = stack(basis(fact))
            Π = rayleighquotient(fact)
            if dot(abs.(@view U[:, 1]), ones(Float64, size(P)[1])'
                            * abs.(A * Π - P * A)) <= ε
                break
            end
        end
        if max_size == 1
            break
        end
        if max_size != k
            fact = expand!(iter, fact)
        end
    end
    A = stack(basis(fact))
    Π = rayleighquotient(fact)
    π_st = @view U[:, 1]
    π_0 = Float64[norm(p_0, 2); zeros(Float64, k-1)]
    return Π, A, π_st, π_0
end
\end{verbatim}
\pagebreak
\paragraph{aggregation.jl}
\begin{verbatim}
using LinearAlgebra

abstract type Aggregation end

"""
    ArnoldiAggregation

Save all current information about an aggregation.

Include all variables which uniquely define an aggregation. Note
that transient distributions are manipulated in-place, so no
"history" is available.

* `P`: Transition matrix
* `p_0`: transient distribution
* `tmp_p_k`: preallocated temporary storage
* `Π`: aggregated step matrix
* `π_st`: aggregated stationary distribution
* `π_k`: aggregated transient distribution
* `tmp_π_k`: preallocated temporary storage
* `A`: disaggregation matrix
* `p̃_st`: approximated stationary distribution
* `p̃_k`: approximated transient distribution
* `tmp_p̃_k`: preallocated temporary storage
* `e`: static error
* `e_k`: dynamic error
* `e_k_bnd`: dynamic error bound
* `e_st`: error of `p̃_st` not being invariant under `P`
* `e_π_st`: ⟨|π|, |ΠA-AP|⋅1_n⟩
* `diff`: |ΠA-AP|
"""
mutable struct ArnoldiAggregation <: Aggregation
    P::AbstractMatrix{Float64}
    p_k::Vector{Float64}
    tmp_p_k::Vector{Float64}
    Π::Matrix{Float64}
    π_st::Vector{Float64}
    π_k::Vector{Float64}
    tmp_π_k::Vector{Float64}
    A::Matrix{Float64}
    p̃_st::Vector{Float64}
    p̃_k::Vector{Float64}
    tmp_p̃_k::Vector{Float64}
    e::Float64
    e_k::Float64
    e_k_bnd::Float64
    e_st::Float64
    e_π_st::Float64
    diff::Matrix{Float64}
end

"""
    ArnoldiAggregation(P::AbstractMatrix, p_0::AbstractVector,
                                algo::Function)::ArnoldiAggregation

Constructor for the `ArnoldiAggregation` struct. Calculate the
aggregation with the given algorithm `algo` using the transition
matrix `P` and initial distribution `p_0`.
Further calculates many other important values for evaluation.
"""
function ArnoldiAggregation(P::AbstractMatrix{Float64},
                p_0::Vector{Float64}, algo::Function)::ArnoldiAggregation
    P = P'  # Transpose, as right hand vector-multiplication is used
    Π, A, π_st, π_0 = algo(P, p_0)
    π_st .*= 1.0 / norm(A * π_st, 1)
    p̃_st = A * π_st
    diff = abs.(A * Π - P * A)
    e = opnorm(A * Π - P * A, 1)
    e_st = norm(p̃_st - P * p̃_st, 1)
    e_π_st = dot(abs.(π_st), ones(Float64, size(P)[1])' * diff)
    return ArnoldiAggregation(P, p_0, copy(p_0), Π, π_st, π_0, copy(π_0),
                                A, p̃_st, copy(p_0), copy(π_0), e, 0.0,
                                0.0, e_st, e_π_st, diff)
end

"""
    step!(aggregation::ArnoldiAggregation)

Step to the next aggregated transient distribution

Uses optimized in-place BLAS-operations internally.
"""
function step!(aggregation::ArnoldiAggregation)
    mul!(aggregation.tmp_π_k, aggregation.Π, aggregation.π_k)
    # Rearrange pointers for consistency in further steps
    aggregation.π_k, aggregation.tmp_π_k, aggregation.tmp_p̃_k =
                aggregation.tmp_π_k, aggregation.π_k, aggregation.tmp_π_k
end

"""
    step_all!(aggregation::ArnoldiAggregation)

Step to the next transient and aggregated transient distribution and
compute current dynamic error bound.

Uses optimized in-place BLAS-operations internally.
"""
function step_all!(aggregation::ArnoldiAggregation)
    mul!(aggregation.tmp_π_k, aggregation.Π, aggregation.π_k)
    mul!(aggregation.tmp_p_k, aggregation.P, aggregation.p_k)
    # Rearrange pointers for consistency in further steps
    aggregation.π_k, aggregation.tmp_π_k, aggregation.tmp_p̃_k =
                aggregation.tmp_π_k, aggregation.π_k, aggregation.tmp_π_k
    aggregation.p_k, aggregation.tmp_p_k =
                aggregation.tmp_p_k, aggregation.p_k

    aggregation.e_k_bnd += dot(abs.(aggregation.π_k),
                ones(Float64, size(aggregation.P)[1])' * aggregation.diff)
end

"""
    getDynamicError!(aggregation::ArnoldiAggregation, norm_mode::Int)

Calculate the current dynamic error and call `step!()` then. If `norm_mode`
is 1, we always normalize `p̃_k`, if it is 0, we only normalize if we know
the result to be better, and in all other cases we don't normalize at all.
"""
function getDynamicError!(aggregation::ArnoldiAggregation, norm_mode::Int)
    mul!(aggregation.p̃_k, aggregation.A, aggregation.tmp_p̃_k)
    if norm_mode == 0
        _cond_l1norm_normalize!(aggregation.p̃_k)
    elseif norm_mode == 1
        _l1norm_normalize!(aggregation.p̃_k)
    end
    aggregation.e_k = _l1norm_diff(aggregation.p̃_k, aggregation.p_k)
    step_all!(aggregation)
end

#=
All functions below are hand-rolled implementations of linear algebra
functionalities. This hand-rolling is done to improve performance
and enable in-place calculations to prevent costly allocations.
=#
function _l1norm_normalize!(a::Vector{Float64})
    s::Float64 = 0.0
    @inbounds @simd for i in eachindex(a)
        s += abs(a[i])
    end
    a ./= s
end

function _cond_l1norm_normalize!(a::Vector{Float64})
    ε::Float64 = 1e-6   # Tolerance for inequalities
    s::Float64 = 0.0
    # Checks if there is an entry <= 1 or >= 1.125.
    single_flag::Bool = false
    # Checks if all entries are negative
    all_flag::Bool = true
    @inbounds for i in eachindex(a)
        if !single_flag && all_flag
            if a[i] <= -1 - ε || a[i] >= 1.125 + ε
                single_flag = true
            end
            if a[i] >= -ε
                all_flag = false
            end
        else
            break
        end
    end
    @inbounds @simd for i in eachindex(a)
        s += abs(a[i])
    end
    if single_flag || (all_flag && s >= 1 - ε) || s >= 2 - ε
        a ./= s
    else
        @inbounds for i in eachindex(a)
            tmp_s = s - a[i]
            if tmp_s <= -1 - ε
                a ./= s
                break
            end
        end
    end
end

function _l1norm_diff(a::Vector{Float64}, b::Vector{Float64})::Float64
    s::Float64 = 0.0
    @inbounds @simd for i in eachindex(a, b)
        s += abs(a[i] - b[i])
    end
    return s
end
\end{verbatim}
